# Supplementary material for: FM-SIREN & FM-FINER: Implicit Neural Representation Using Nyquist-based Orthogonality
Source: arXiv:2509.23438 source file (2026-04-11)
Supplement: Supplementary file 1 [file NeRF.tex]

\subsection{Neural Radiance Fields}

\par NeRF synthesizes novel 3D scene views from sparse 2D images by learning a continuous volumetric representation optimized via ray-based rendering \cite{mildenhall2020nerfrepresentingscenesneural}. In our experiments, the volume is discretized at a resolution of $100 \times 100 \times 100$, corresponding to a Nyquist frequency of $50$ cycles/volume. We adopt the concise implementation of \cite{vandegar2025nerf100lines} on the Blender dataset \cite{mildenhall2021nerf}, using networks with five layers that model density and color. Performance is evaluated as the average PSNR across all 200 test images per scene, each at a resolution of $400 \times 400$. As reported in Table~\ref{tab:NeRF} and illustrated in Figure~\ref{fig:NeRF}, FM-SIREN and FM-FINER achieve higher PSNR than baseline models in most scenes. Although the improvements in reconstruction quality are modest, both FM-SIREN and FM-FINER reduce compute time by $14.53\%$ and $17.06\%$, respectively, demonstrating the efficiency gains of our approach.

\begin{figure}[t]
    \centering
    % Row 1
    \begin{subfigure}{0.22\textwidth}
        \includegraphics[width=\linewidth]{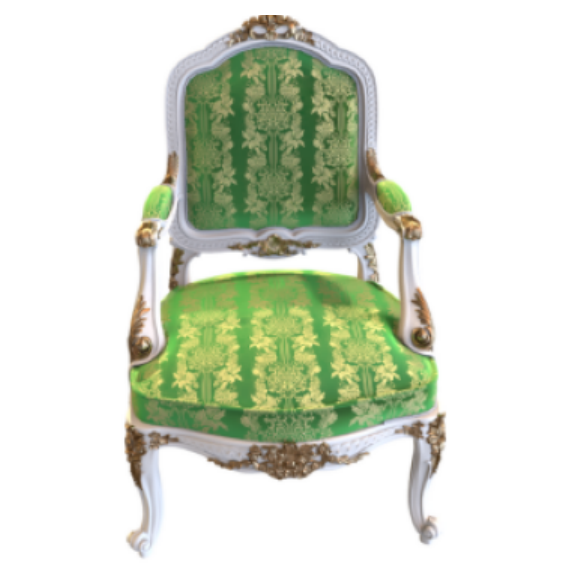}
        \caption{Ground Truth}
    \end{subfigure}
    \begin{subfigure}{0.22\textwidth}
        \includegraphics[width=\linewidth]{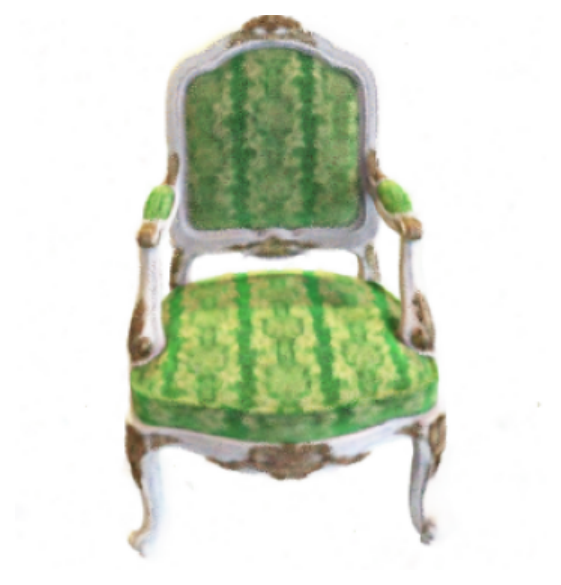}
        \caption{SIREN}
    \end{subfigure}
    \begin{subfigure}{0.22\textwidth}
        \includegraphics[width=\linewidth]{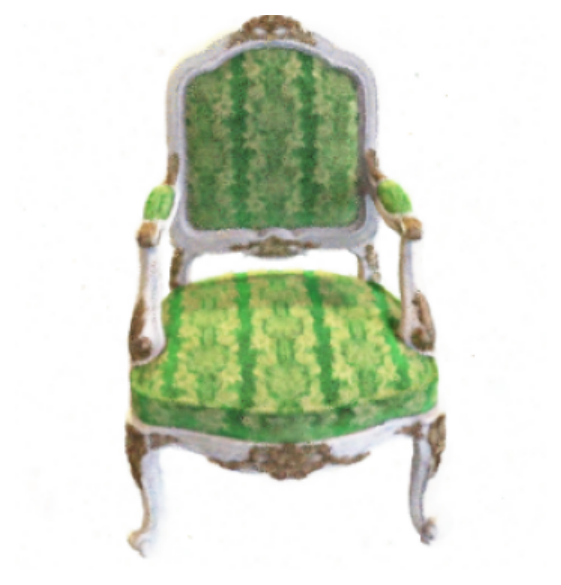}
        \caption{FINER}
    \end{subfigure}
    \begin{subfigure}{0.22\textwidth}
        \includegraphics[width=\linewidth]{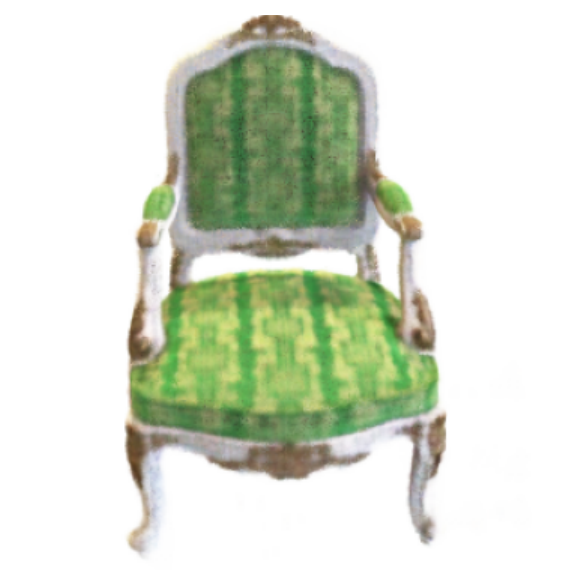}
        \caption{PE}
    \end{subfigure}

    % Row 2
    \begin{subfigure}{0.22\textwidth}
        \includegraphics[width=\linewidth]{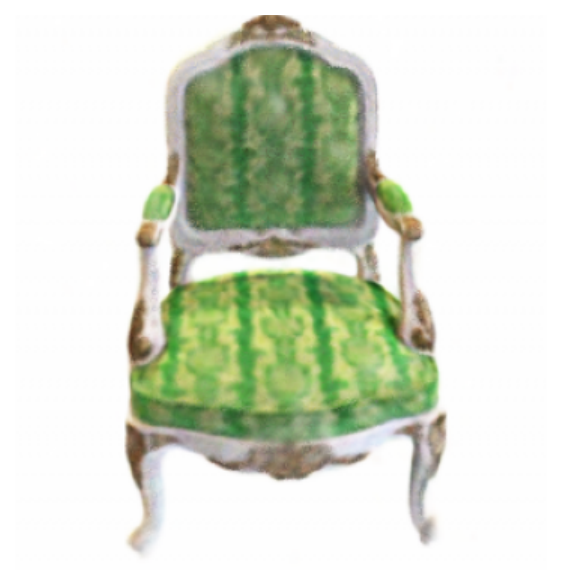}
        \caption{GAUSS}
    \end{subfigure}
    \begin{subfigure}{0.22\textwidth}
        \includegraphics[width=\linewidth]{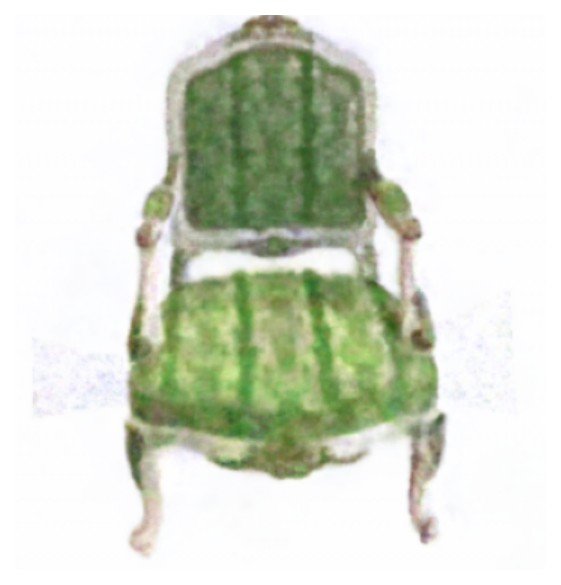}
        \caption{WIRE}
    \end{subfigure}
    \begin{subfigure}{0.22\textwidth}
        \includegraphics[width=\linewidth]{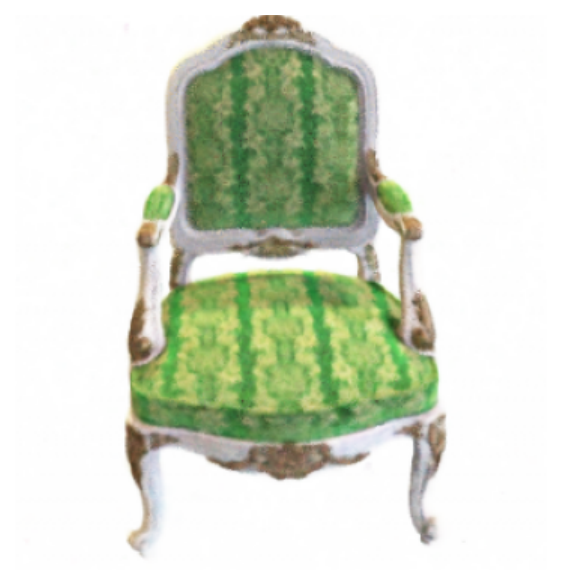}
        \caption{FM-SIREN}
    \end{subfigure}
    \begin{subfigure}{0.22\textwidth}
        \includegraphics[width=\linewidth]{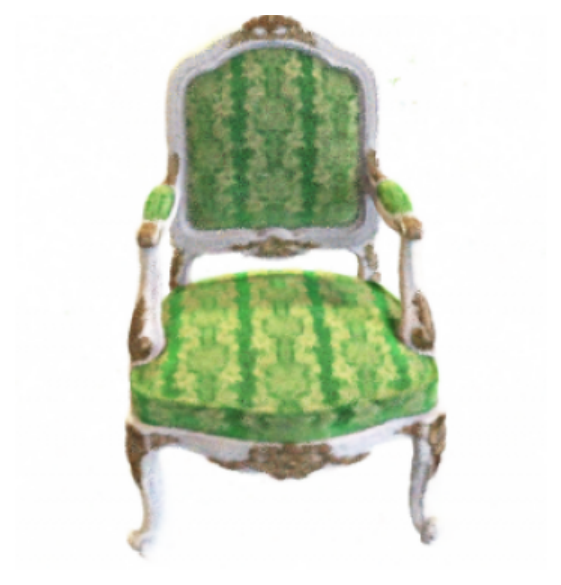}
        \caption{FM-FINER}
    \end{subfigure}
    \vspace{-5pt}
    \caption{Qualitative reconstruction results of the Chair scene from the Blender dataset \cite{mildenhall2021nerf}, using five-layer networks (three layers for the first block, one layer for density, and one layer for color). FM-SIREN and FM-FINER achieve improvements over the baselines, with exact PSNR values reported in Table~\ref{tab:NeRF}.}
    \vspace{-10pt}

    \label{fig:NeRF}
\end{figure}

\begin{table}[h!]
    \centering
    \caption{Epoch time, number of parameters, and PSNR for NeRF fitting on the Blender dataset \cite{mildenhall2021nerf}. \colorbox{Goldenrod}{Best} and \colorbox{Dandelion}{Second Best} results are highlighted.}
    \vspace{-5pt}
    \resizebox{1\textwidth}{!}{%
    \begin{tabular}{@{}lc ccccccccc@{}}
        \toprule
        \multirow{2}{*}{\textbf{Model}} & 
        \multirow{2}{*}{\textbf{Epoch Time (s)}} & 
        \multirow{2}{*}{\textbf{Parameters}} & 
        \multicolumn{8}{c}{\textbf{PSNR} $\uparrow$} \\
        \cmidrule(lr){4-11}
         & & & \textbf{Lego} & \textbf{Ship} & \textbf{Chair} & \textbf{Mic} & \textbf{Materials} & \textbf{Hotdog} & \textbf{Ficus} & \textbf{Drums} \\
        \midrule
        FINER & $106.84$ & $199,428$ & \colorbox{Dandelion}{$28.01$} & $33.09$ & $34.53$ & $34.44$ & $33.38$ & $37.16$ & $33.75$ & $32.51$ \\
        GAUSS & $98.68$ & $199,428$ & $27.58$ & $32.91$ & $34.23$ & \colorbox{Dandelion}{$34.48$} & $33.21$ & $36.66$ & $33.33$ & $32.31$ \\
        Positional Encoding & $126.33$ & $214,788$ & $27.63$ & $32.48$ & $34.13$ & $34.24$ & $32.86$ & $36.17$ & $32.82$ & $31.72$ \\
        SIREN & $122.12$ & $199,428$ & $27.81$ & $33.08$ & $34.42$ & $34.45$ & $33.38$ & $37.00$ & \colorbox{Goldenrod}{$33.79$} & $32.48$ \\
        WIRE & $140.04$ & $199,428$ & $23.36$ & $20.34$ & $25.21$ & $26.31$ & $23.07$ & $27.50$ & $23.19$ & $21.11$ \\
        \midrule
        \textbf{FM-SIREN} & $104.37$ & $199,428$ & $27.55$ & \colorbox{Goldenrod}{$33.17$} & \colorbox{Dandelion}{$34.55$} & \colorbox{Goldenrod}{$34.64$} & \colorbox{Goldenrod}{$33.45$} & \colorbox{Dandelion}{$37.37$} & \colorbox{Dandelion}{$33.76$} & \colorbox{Goldenrod}{$32.54$} \\
        \textbf{FM-FINER} & $88.61$ & $199,428$ & \colorbox{Goldenrod}{$28.11$} & \colorbox{Dandelion}{$33.14$} & \colorbox{Goldenrod}{$34.56$} & $29.81$ & \colorbox{Dandelion}{$33.41$} & \colorbox{Goldenrod}{$37.41$} & $33.73$ & \colorbox{Dandelion}{$32.53$} \\
        \bottomrule
    \end{tabular}%
    }
    \label{tab:NeRF}
\end{table}
